# Supplementary material for: Cosmological Predictions from the Primordial Universe: Non-Gaussianities
Source: arXiv:1803.01759 source file (2018-03-05)
Supplement: Supplementary file 1 [file AppendixA.tex]

% Appendix A

\chapter{Appendix A.} % Main appendix title

\label{AppendixA} % For referencing this appendix elsewhere, use \ref{AppendixA}

\lhead{Appendix A. \emph{A}} % This is for the header on each page - perhaps a shortened title

Parameter conventions:\\

$\epsilon = \frac{\dot{H}}{H^2}.$
